# Supplementary material for: Soft mode induced structural phase transition in Ba$_2$ZnTeO$_6$ at high pressure
Source: arXiv:2503.11971 ancillary file (2025-03-15)
Supplement: Supplementary file 1 [file Supplementary_unmarked.pdf]

# Supplementary: Soft mode induced structural phase transition in $\text{Ba}_2\text{ZnTeO}_6$ at high pressure

Bidisha Mukherjee,<sup>1,2</sup> Surajit Adhikari,<sup>3</sup> Mrinmay Sahu,<sup>1,2</sup> Asish Kumar Mishra,<sup>1,2</sup>  
Bhagyashri Giri,<sup>1,2</sup> Priya Johari,<sup>3</sup> Konstantin Glazyrin,<sup>4</sup> and Goutam Dev Mukherjee<sup>1,2,\*</sup>

<sup>1</sup>*Department of Physical Sciences, Indian Institute of Science  
Education and Research Kolkata, Mohanpur Campus,  
Mohanpur 741246, Nadia, West Bengal, India.*

<sup>2</sup>*National Centre for High-Pressure Studies,  
Indian Institute of Science Education and Research Kolkata,  
Mohanpur Campus, Mohanpur 741246, Nadia, West Bengal, India.*

<sup>3</sup>*Department of Physics, School of Natural Sciences,  
Shiv Nadar Institution of Eminence, Greater Noida,  
Gautam Buddha Nagar, Uttar Pradesh 201314, India.*

<sup>4</sup>*Photon Science, Deutsches Elektronen Synchrotron, 22607 Hamburg, Germany*

(Dated: March 11, 2025)

## I. FESEM IMAGES

We observed the microstructure of BZTO powder using SUPRA 55 VP- 4132 CARL ZEISS FESEM running at 5.21 KeV. We have estimated the grain size and their distribution from the different positions of the sample (FIG. S1).

## II. BOND ANGLE VARIANCE

We checked the pressure evolution of bond angle variance. The bond angle variance of a polyhedron measures how much the bond angles within the polyhedron deviate from the ideal geometry of that polyhedron. For example, in the case of a perfect octahedron, the bond angles should be  $90^\circ$ , and any deviation from that will be reflected in bond angle variance. In other words, it quantifies the degree of distortion from the ideal bond angles. The variation of bond angle variance with pressure for  $\text{Te}(1)\text{O}_6$  and  $\text{Te}(2)\text{O}_6$  octahedra is shown in FIG. S6. Bond angle variance increases linearly with increasing pressure up to 5 GPa with an average rate of about  $0.007 \text{ GPa}^{-1}$  then remains almost constant up to 7.5 GPa but with further compression it increases rapidly with pressure. Greater bond angle variance is correlated with decreased structural stability. The decrease in structural stability is also reflected in the pressure dependency of FWHM of the Raman modes and softening of the  $N_1$  mode as mentioned in the earlier section. So it can be inferred that the anomalous increase in bond angle variance and structural trigonality are the key causes of making the sample unstable above 7.5 GPa and the same is reflected in the pressure evolution of Raman modes.

## III. ABSORPTION SPECTRA MEASUREMENT

To investigate the electronic properties of BZTO we have measured its absorption spectra at ambient conditions. The absorbance (A) versus wavelength data is shown in FIG. S7 (a). Then we have plotted  $(Ah\nu)^n$  versus  $h\nu$ , where  $n = 2$  is applicable for direct band gap semiconductors and  $n = \frac{1}{2}$  is applicable for indirect band gap semiconductors and  $h\nu$  is the photon's energy (see FIG. S7 (b)). Now we take the help of the Tauc formula to estimate

---

\* Corresponding author: goutamdev@iiserkol.ac.in

the value of optical direct and indirect bandgap which is:  $(Ah\nu)^n = C(h\nu - E_g)$ . We used this equation to fit the linear absorption edge; where  $C$  is a constant, and  $E_g$  is the optical bandgap. The optical indirect bandgap is measured to be 3.52(1) eV at ambient conditions revealing that the sample is an indirect bandgap semiconductor.

#### IV. ADDITIONAL DFT RESULTS

For DFT calculations of both the phases we have used experimental lattice parameters as the starting model. The lattice constants and atomic positions were fully optimized. The resulting values of lattice parameters at different pressure points and average bond lengths of different octahedra are tabulated below in TABLE S1 ( $R\bar{3}m$  phase) and TABLE S2 ( $C2/m$  phase).

| Pressure<br>(GPa) | Lattice parameters |       | Average bond lengths |             |             |
|-------------------|--------------------|-------|----------------------|-------------|-------------|
|                   | a (Å)/ b (Å)       | c (Å) | Zn-O (Å)             | Te(1)-O (Å) | Te(2)-O (Å) |
| 0                 | 5.92               | 29.14 | 2.15                 | 1.96        | 1.96        |
| 5                 | 5.83               | 28.73 | 2.12                 | 1.94        | 1.95        |
| 10                | 5.75               | 28.42 | 2.1                  | 1.92        | 1.94        |
| 12                | 5.72               | 28.30 | 2.09                 | 1.92        | 1.94        |
| 18                | 5.65               | 27.99 | 2.07                 | 1.9         | 1.93        |
| 24                | 5.59               | 27.75 | 2.05                 | 1.89        | 1.92        |
| 41.2              | 5.45               | 27.14 | 2                    | 1.86        | 1.91        |

TABLE S1: Values of lattice parameters and average bond lengths of various octahedra at different pressure points for  $R\bar{3}m$  space group.

| Pressure<br>(GPa) | Lattice parameters |       |       |             | Average bond lengths |             |             |
|-------------------|--------------------|-------|-------|-------------|----------------------|-------------|-------------|
|                   | a (Å)              | b (Å) | c (Å) | $\beta$ (°) | Zn-O (Å)             | Te(1)-O (Å) | Te(2)-O (Å) |
| 0                 | 10.23              | 5.9   | 10.29 | 106.66      | 2.16                 | 1.96        | 1.96        |
| 5                 | 10.07              | 5.82  | 10.17 | 106.84      | 2.13                 | 1.94        | 1.95        |
| 10                | 9.94               | 5.75  | 10.07 | 106.89      | 2.10                 | 1.93        | 1.94        |
| 12                | 9.9                | 5.72  | 10.03 | 106.93      | 2.09                 | 1.92        | 1.94        |
| 18                | 9.78               | 5.65  | 9.92  | 106.94      | 2.06                 | 1.90        | 1.93        |
| 24                | 9.67               | 5.59  | 9.83  | 106.96      | 2.04                 | 1.89        | 1.92        |
| 41.2              | 9.42               | 5.45  | 9.63  | 106.96      | 1.99                 | 1.86        | 1.91        |

TABLE S2: Values of lattice parameters and average bond lengths of various octahedra at different pressure points for  $C2/m$  space group.

## V. FIGURES

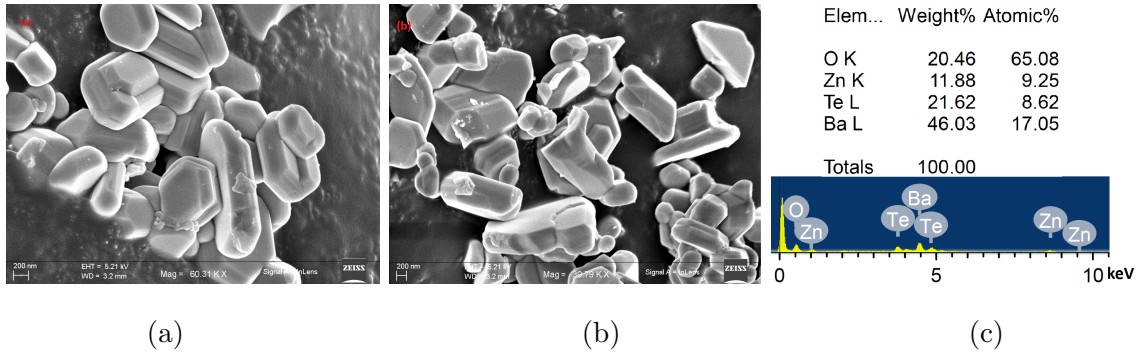

FIG. S1: (a), (b) SEM image at two different positions of powder BZTO sample. (c) EDX spectra with atomic percentage.

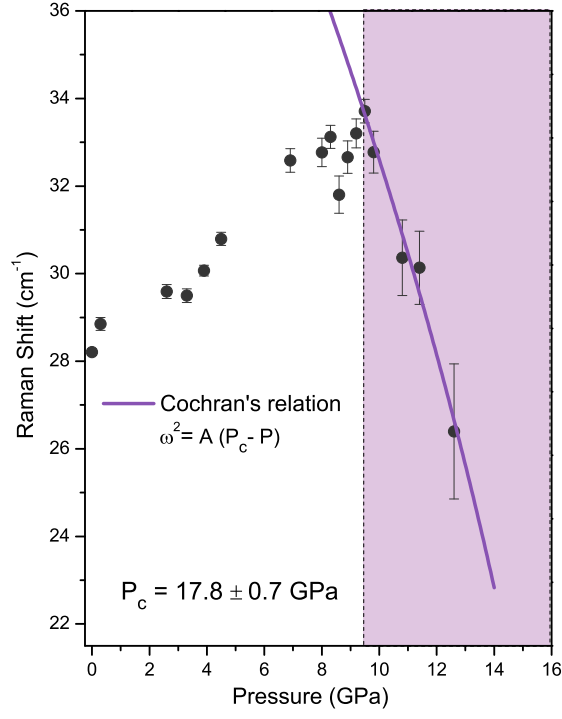

FIG. S2: Pressure evolution of soft mode frequency. Black solid circles represent experimental data and the violet line is the theoretical fit to it which results in  $P_c = 17.8 \pm 0.7$  GPa.

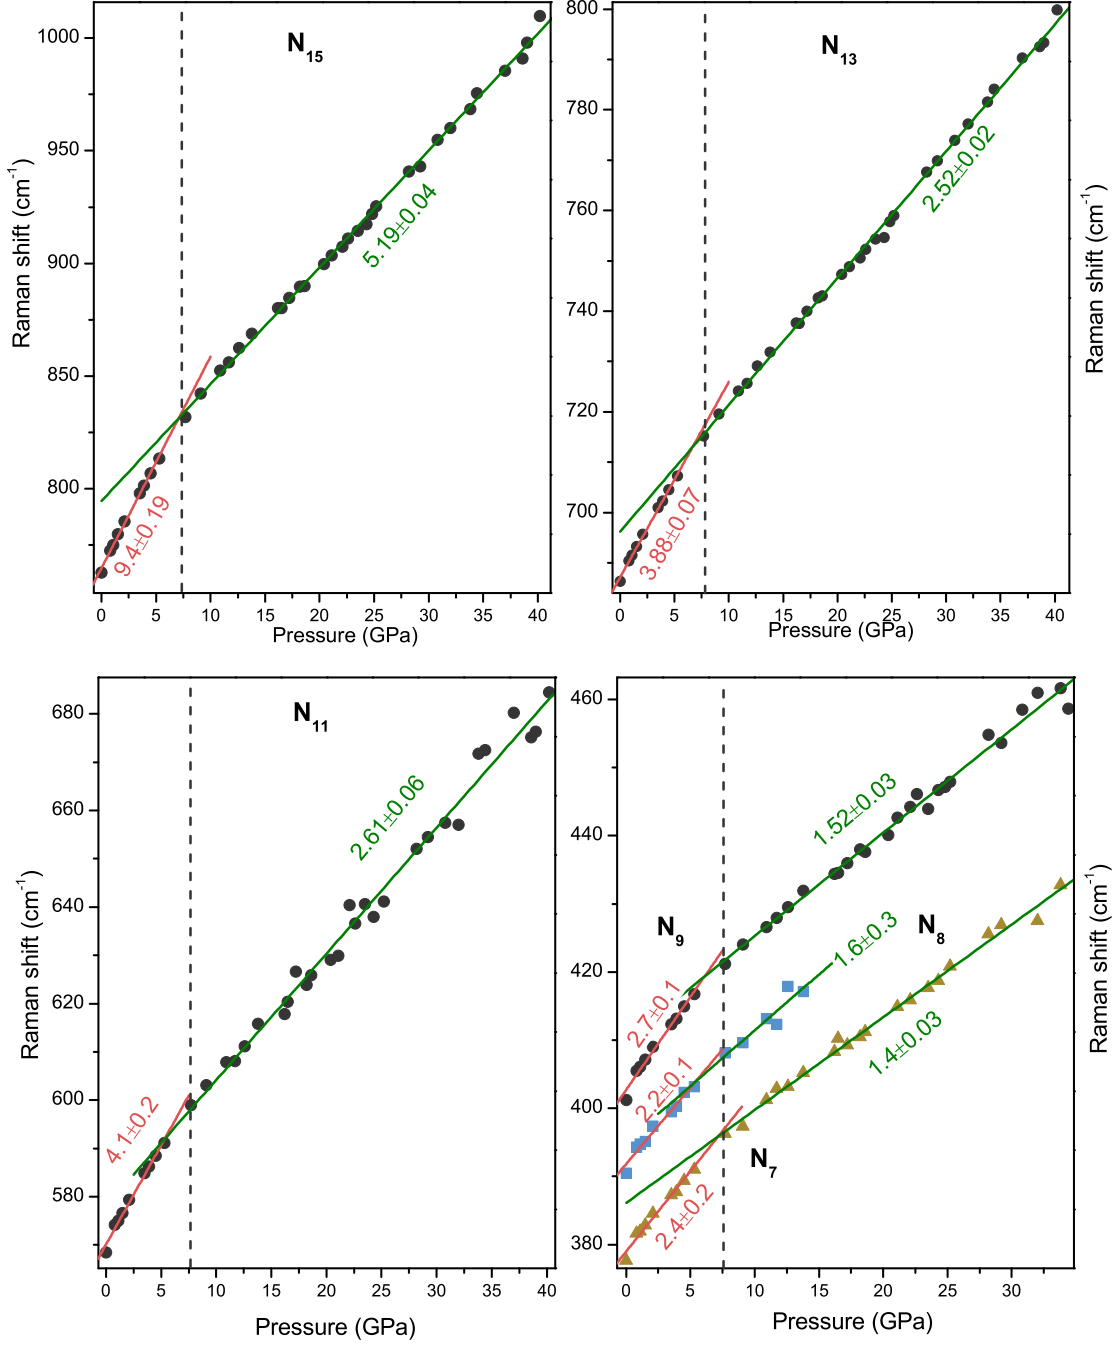

FIG. S3: Pressure evolution of the frequencies of some prominent phonon mode. The data points represent the experimental data and the solid lines are the theoretical fit to it. The resulting slope values are mentioned with each fitting and are in cm<sup>-1</sup>GPa<sup>-1</sup>.

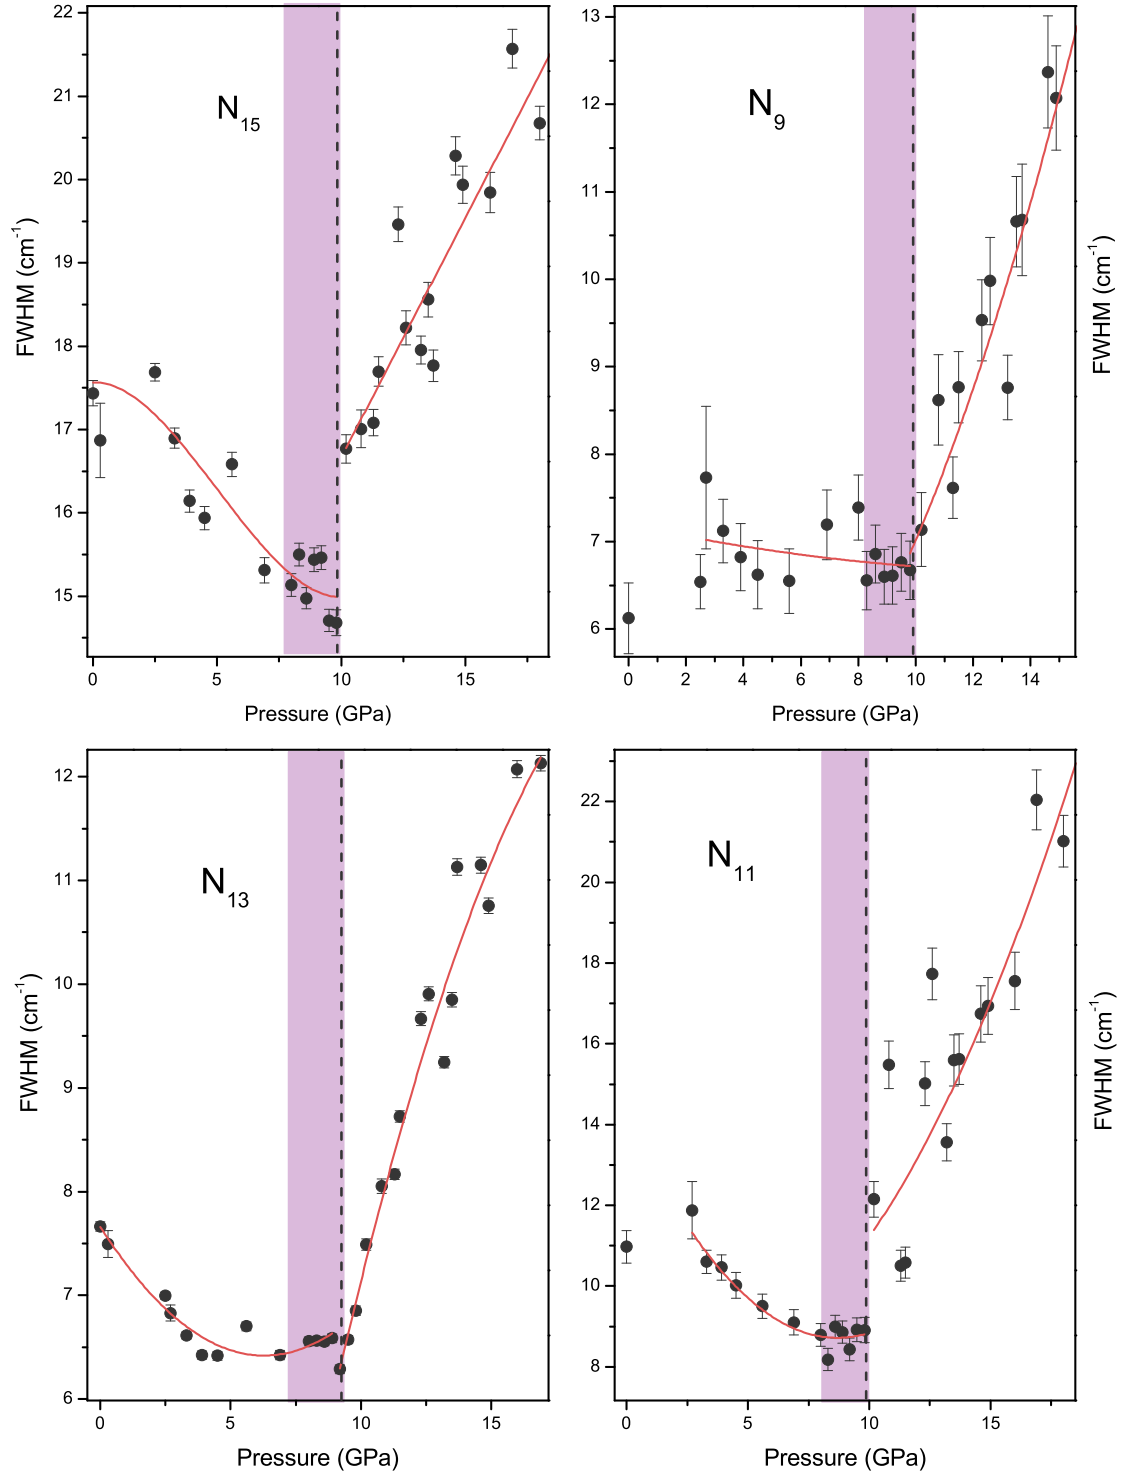

FIG. S4: Pressure evolution of FWHM of N<sub>15</sub>, N<sub>9</sub>, N<sub>13</sub> and N<sub>11</sub> modes.

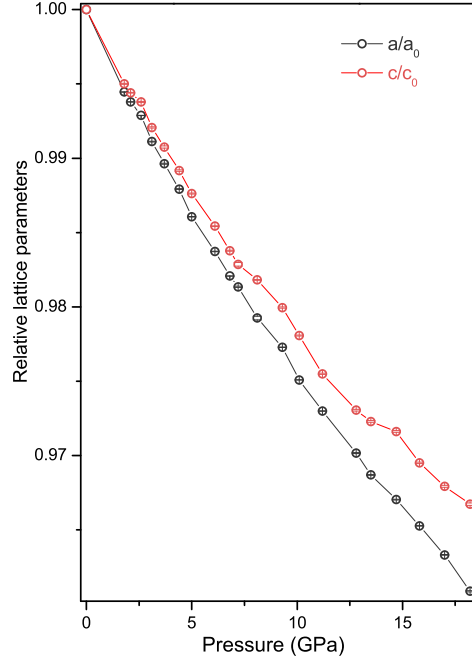

FIG. S5: Response of relative lattice parameters by applying pressure.  $a_0$  and  $c_0$  are the lattice parameters of ambient conditions along a-axis and c-axis, respectively.

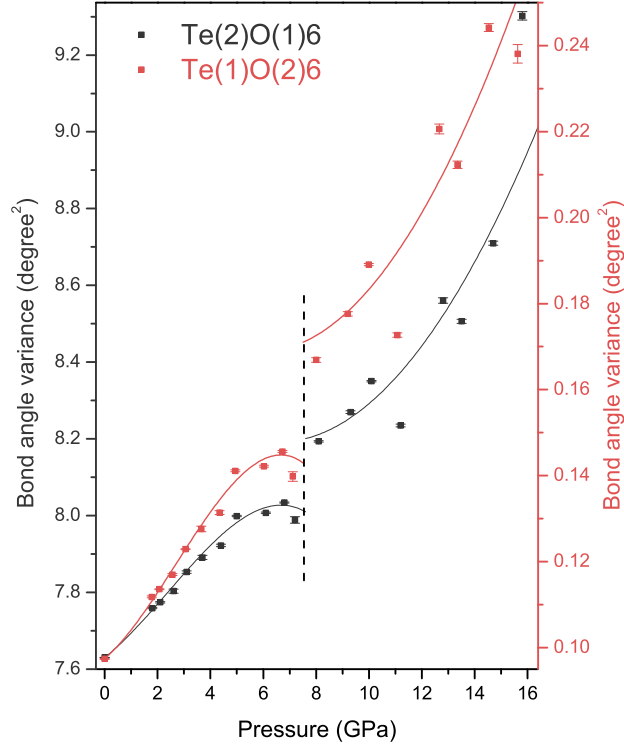

FIG. S6: Variation of bond angle variance of  $\text{TeO}_6$  octahedra as a function of pressure. The dashed line indicates sudden jump of the bond angle variance in response to pressure.

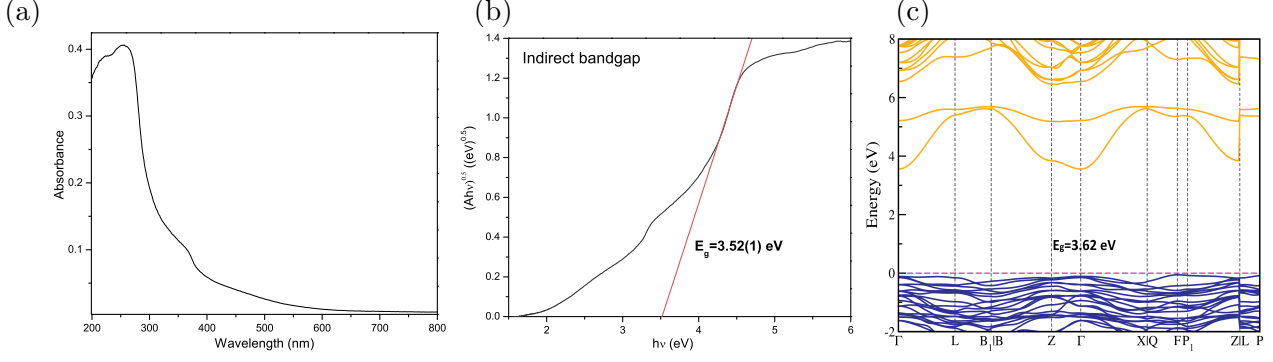

FIG. S7: (a) The absorbance versus wavelength data and (b) Tauc's plot of indirect bandgap of BZTO using UV-visible spectrum at ambient conditions. (c) Calculated bandstructure of BZTO at ambient conditions using HSE06 xc functional.

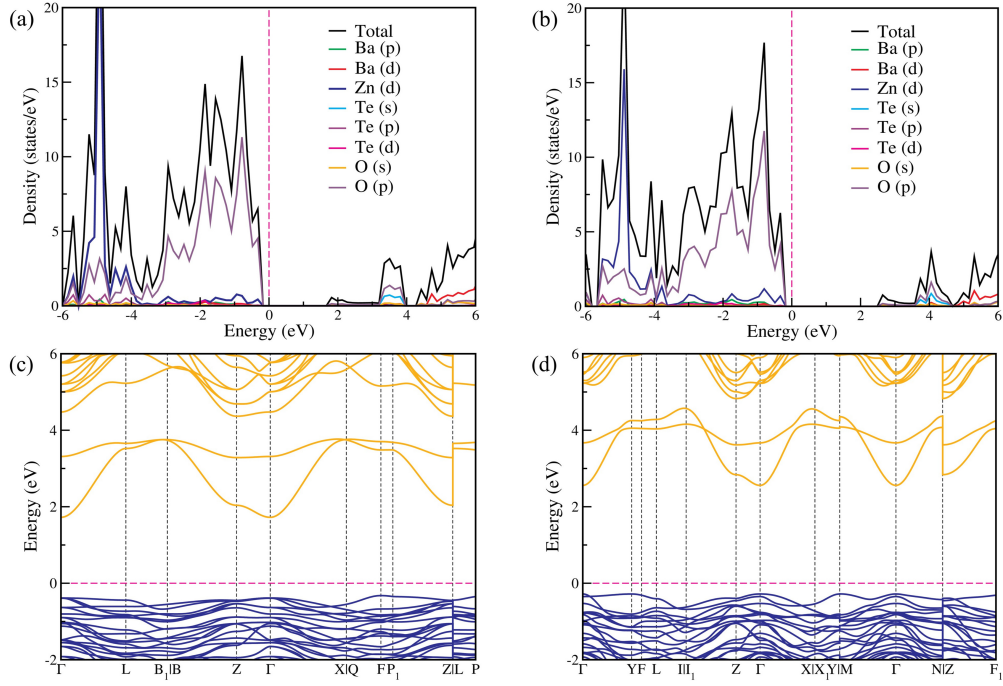

FIG. S8: Calculated (a, b) atom-projected partial density of states (pDOS) and (c, d) electronic band structures of trigonal phase at ambient conditions (left) and monoclinic phase at 24 GPa (right) respectively for Ba<sub>2</sub>ZnTeO<sub>6</sub> crystal structure obtained using PBE xc functional.
